# Supplementary material for: Anisotropic diffusion of radiation-induced self-interstitial clusters in HCP zirconium: a molecular dynamics and rate-theory assessment
Source: arXiv:2309.05781 source file (2023-09-11)
Supplement: Supplementary file 1 [file Caption.tex]

\documentclass[11pt,a4paper,roman]{moderncv}
\begin{document}

Video1.mp4\\
A single self-interstitial atom (SIA) is added near a cluster of 6 SIAs and merges in the first frame (00:00). The 7-SIA cluster moves in all directions with preferential glide on the basal plane. To better show the glide, the timestep is increased from 500 fs to 50 ps after 200 frames (00:20). This MD simulation is performed in LAMMPS using M3R for pure Zr at 573K followed by Wigner-Seitz cell analysis. This video is rendered in OVITO along the basal plane [1-210] (X direction in a Cartesian coordinate system with its Z along the c direction).\\

Video2.mp4\\
A primary knock-on (PKA) atom with an energy of 10 keV creates a cascade in pure Zr at 573K. Here, the red and blue balls represent the single self-interstitial atoms (SIAs) and vacancies, respectively. In this video, a cluster of 5 SIAs merges with a single SIA making a cluster of 6 SIAs that rapidly glides on the basal plane along the closed-pack direction until it merges with another single SIA. The resultant cluster of 7 SIAs then merges with the adjacent cluster of 10 vacancies, leaving a cluster of 3 vacancies behind. This MD simulation was performed in LAMMPS using M3R and visualized after Wigner-Seitz cell analysis. The video was rendered in OVITO and viewed along the normal direction of the basal plane.\\

Video3.mp4\\
Using the equivalent sphere analysis, the diffusion of a self-interstitial atom (SIA) and its subsequent SIA-cluster interaction is captured in this video. Here, the blue, yellow and red balls are surplus, empty and distorted positions.\\

SIACB.m\\
Self-interstitial atom cluster bias (SIACB) model to be used in MATLAB. All the credit goes to the original authors A. V. Barashev, S. I. Golubov, R. E. Stoller.

M2R.eampot\\
M. I. Mendelev, G. J. Ackland's EAM potential No.2 after reparameterization (M2R)

M3R.eampot\\
M. I. Mendelev, G. J. Ackland's EAM potential No.3 after reparameterization (M3R)

SM.tex
**Abstract of SM
\end{document}
